# Supplementary material for: MedEvoEval: Evaluating Continual Evolution of Doctor Agents through Simulated Clinical Episodes
Source: arXiv:2606.28900 source file (2026-10-18)
Supplement: Supplementary file 1 [file supplement_appendix.tex]

\section{Artifact Inventory and Responsible Use}
\label{app:artifact}

This appendix documents the released executable evaluation artifact for \textsc{MedEvoEval}. The artifact contains the \texttt{src/medevoeval} Python package, experiment configurations, six JSON schemas, the \textsc{Chinese MedEvoEval-MedQA-700} dataset release, sanitized process trajectories and step-level records, manifests, Croissant metadata, cached aggregate results, reproduction scripts, audit documentation, and example outputs.

\begin{table}[!htbp]
\centering
\caption{Released evaluation artifact contents.}
\label{tab:app_release_boundary}
\small
\begin{tabular}{p{0.30\linewidth}p{0.58\linewidth}}
\toprule
Released component & Purpose \\
\midrule
\textsc{Chinese MedEvoEval-MedQA-700} & 700 release-safe Chinese MedQA-derived simulated clinical cases with stable release IDs. \\
Training-oriented process records & 3,103 sanitized complete-episode trajectories and 3,386 high-quality single-step decision samples. \\
\texttt{src/medevoeval} package & Minimal runner, action space, patient simulator, exam service, doctor/consultant agents, judge, scoring, memory, statistics, and analysis helpers. \\
Experiment configurations & Demo, benchmark, MDT, continual-memory, update/stability, and live-API configuration files. \\
Schemas, manifests, and Croissant metadata & Validate case, episode, event-log, score, memory, and process files; document release rows, source boundaries, and Responsible AI metadata. \\
Cached metrics, scripts, and audit docs & Recompute paired tests, reproduce table CSVs and figure source data, check splits, validate the package, and inspect audit notes. \\
Example outputs & Inspect demo episodes, event logs, score rows, cached tables, figure data, and live-check examples. \\
\bottomrule
\end{tabular}
\end{table}

\paragraph{Training-oriented derivatives.}
In addition to the 700 benchmark episodes, the artifact includes derived training files for agent-policy research. The complete-episode derivative contains 3,103 trajectory records, each corresponding to a full episode. The file \texttt{chinese\_medevoeval\_process\_steps.jsonl} contains 3,386 single-step decision samples extracted from high-quality episodes. Each step records the current context, previous questions and tests, available actions, the target action, the target output text, and the final episode score. These samples are intended for supervised fine-tuning, behavior cloning, or action-policy training on what to ask, test, or finalize next. Low-scoring or failed episodes are excluded from the step file to avoid treating poor decisions as positive training targets.

\paragraph{Responsible use.}
\textsc{MedEvoEval} is a simulation-based evaluation framework for research use. It does \emph{not} constitute clinical validation, medical-device certification, or evidence that an evaluated agent is safe for real-world deployment. The released episodes, logs, and code are intended for benchmark inspection and reproducibility, not for real clinical decisions.

\section{Executable Episode Protocol Details}
\label{app:protocol_details}

This appendix groups the executable protocol details used by the runner: the role-specific case schema, runtime prompt templates, the doctor structured-output template, and a compact memory-record example.

\subsection{Role-Specific Case Schema}
\label{app:schema}

The implementation defines an episode case as a structured object with patient, examination, and manager views. The doctor-facing state is derived from this object and exposes only an opening instruction, revealed history, returned tests, optional consultant notes, optional retrieved memory cards, and the allowed test catalog. Figure~\ref{fig:app_role_views} summarizes the role-specific visibility constraints, and the synthetic sample illustrates the case format.

\begin{figure}[!htbp]
\centering
\begin{tikzpicture}[
  font=\small,
  box/.style={draw, rounded corners=2pt, align=center, minimum width=3.2cm, minimum height=1cm},
  note/.style={draw, rounded corners=2pt, align=left, minimum width=4.0cm, inner sep=4pt},
  arrow/.style={-Latex, thick}
]
\node[box, fill=gray!10] (case) at (0,0) {Structured case};
\node[box, fill=blue!8] (patient) at (-4,-2) {PatientView\\patient simulator};
\node[box, fill=green!8] (exam) at (0,-2) {ExamView\\exam service};
\node[box, fill=orange!10] (manager) at (4,-2) {ManagerView\\manager judge};
\node[note, fill=purple!7] (doctor) at (0,-4.3) {Doctor sees:\\$\bullet$ opening complaint\\$\bullet$ revealed history\\$\bullet$ returned tests\\$\bullet$ consultant notes (optional)\\$\bullet$ retrieved memory (optional)};
\node[note, fill=red!6] (hidden) at (6.0,-4.3) {Doctor does \emph{not} see:\\$\bullet$ hidden patient facts\\$\bullet$ unrevealed tests\\$\bullet$ manager answer key\\$\bullet$ scoring rubric details};

\draw[arrow] (case) -- (patient);
\draw[arrow] (case) -- (exam);
\draw[arrow] (case) -- (manager);
\draw[arrow] (patient) -- (doctor);
\draw[arrow] (exam) -- (doctor);
\draw[arrow] (manager) -- ++(0,-0.7) -| (hidden.north);
\end{tikzpicture}
\caption{Role-specific case views and visibility constraints. Patient and examination information is revealed only through actions, while manager-side labels and rubrics remain hidden until evaluation.}
\label{fig:app_role_views}
\end{figure}

\paragraph{Synthetic sample.}
The following example is synthetic and only illustrates the format.

\begin{codebox}{Schema B.1: Synthetic case example}
\begin{lstlisting}[language=json]
{
  "case_id": "synthetic_demo_001",
  "source": {"type": "synthetic", "raw_case_id": "demo"},
  "patient_view": {
    "demographics": {"age": 46, "sex": "female"},
    "chief_complaint": "intermittent chest discomfort for two days",
    "history_facts": [
      "pain worsens with exertion",
      "no fever",
      "family history of premature coronary disease"
    ]
  },
  "exam_view": {
    "tests": {
      "electrocardiogram": "nonspecific ST-T changes",
      "troponin": "mildly elevated"
    },
    "test_catalog": ["electrocardiogram", "troponin"]
  },
  "manager_view": {
    "ground_truth": {
      "diagnosis": {
        "display_name": "acute coronary syndrome",
        "acceptable_names": ["ACS"]
      },
      "evidence_rubric": {
        "key_points": ["exertional chest pain", "troponin elevation"]
      },
      "management_rubric": {
        "key_points": ["urgent cardiology evaluation"]
      }
    }
  }
}
\end{lstlisting}
\end{codebox}

\subsection{Prompt Templates}
\label{app:prompts}

\begin{promptbox}{Prompt B.1: Attending-doctor system prompt}
\begin{lstlisting}
You are an outpatient attending doctor in a simulated evaluation episode.
Your goal is to reach a safe diagnosis and plan.
Use only information revealed by the patient, examination service,
consultant, and memory cards in this conversation.

Rules:
1. Output valid JSON only.
2. Choose exactly one action from: ASK, REQUEST_TEST, CALL_MDT, FINALIZE.
3. Do not invent symptoms, examination results, laboratory values,
   imaging findings, or prior diagnoses.
4. REQUEST_TEST must use an exact test_name from the allowed catalog.
5. CALL_MDT may ask for diagnostic advice, but the final decision remains
   your responsibility.
6. FINALIZE only when evidence is sufficient or the turn limit requires
   termination. Provide diagnosis, evidence, plan, and followup.
7. Use retrieved memory cards as experience hints, not as patient facts.

Episode state:
- patient_opening: {patient_opening}
- allowed_tests: {allowed_tests}
- max_total_turns: {max_total_turns}
- max_tests_per_visit: {max_tests_per_visit}
- revealed_history: {revealed_history}
- returned_tests: {returned_tests}
- consultant_notes: {consultant_notes}
- retrieved_memory_cards: {retrieved_memory_cards}
\end{lstlisting}
\end{promptbox}

\begin{promptbox}{Prompt B.2: Patient-simulator prompt}
\begin{lstlisting}
You are a simulated outpatient patient. Answer the question from the
attending doctor using only the hidden patient facts listed below.

Rules:
1. Do not diagnose yourself.
2. Do not reveal examination, laboratory, imaging, or manager-only fields.
3. If the doctor asks about a listed hidden_history_fact, answer directly.
4. If the doctor asks about something not specified, say that you are not
   sure or that you do not recall.
5. Keep the answer natural, brief, and patient-like.
6. Output valid JSON only.

hidden_patient_view:
{patient_view}

doctor_question:
{question}

Return:
{
  "answer": "string",
  "revealed_facts": ["fact id or short fact text"],
  "unanswered_reason": "none|not_in_patient_view|unclear_question"
}
\end{lstlisting}
\end{promptbox}

\begin{promptbox}{Prompt B.3: Examination-service prompt}
\begin{lstlisting}
You are an examination-result service for a simulated outpatient episode.
Return only results that exist in the provided exam_view.

Rules:
1. Match the requested test to the closest allowed catalog item.
2. If there is no allowed match, return returned=false and do not invent a
   result.
3. If the test is available, return the stored result verbatim or as a
   concise paraphrase without adding new findings.
4. Output valid JSON only.

allowed_tests:
{allowed_tests}

exam_view:
{exam_view}

requested_test:
{requested_test}

Return:
{
  "returned": true,
  "matched_test_name": "string",
  "match_type": "exact|alias|none",
  "result": "string",
  "reason": "string"
}
\end{lstlisting}
\end{promptbox}

\begin{promptbox}{Prompt B.4: MDT-consultant prompt}
\begin{lstlisting}
You are an MDT consultant in a simulated diagnostic episode. Provide a
second opinion based only on the revealed patient history, returned tests,
and the current working diagnoses of the attending doctor.

Rules:
1. You cannot order tests directly.
2. You cannot access hidden labels or unrevealed examination results.
3. Recommend at most one next question if more information is needed.
4. If the evidence is sufficient, recommend FINALIZE and give a concise
   diagnosis suggestion.
5. Output valid JSON only.

revealed_context:
{revealed_context}

attending_state:
{attending_state}
\end{lstlisting}
\end{promptbox}

\subsection{Structured Output Templates}
\label{app:structured_outputs}

\begin{codebox}{Template B.1: Doctor structured output}
\begin{lstlisting}[language=json]
{
  "action": "ASK|REQUEST_TEST|CALL_MDT|FINALIZE",
  "utterance": "string",
  "question": "string",
  "test_name": "string",
  "rationale": ["string"],
  "working_diagnoses": ["string"],
  "needs_mdt": false,
  "diagnosis": ["string"],
  "evidence": ["string"],
  "plan": ["string"],
  "followup": ["string"]
}
\end{lstlisting}
\end{codebox}

\subsection{Example Memory Record}
\label{app:event_log}

The following synthetic memory-card example shows the memory-record format without including any third-party-derived case content.

\begin{codebox}{Log B.2: Synthetic memory-card examples}
\begin{lstlisting}[language=json]
[
  {
    "case_id": "synthetic_demo_001",
    "visit_index": 0,
    "memory_type": "success",
    "experience": "Exertional chest discomfort plus biomarker elevation supported early cardiac workup.",
    "rule_text": "IF chest discomfort worsens with exertion THEN ask cardiac-risk questions and prioritize ECG/troponin.",
    "outcome": "accepted diagnosis and supported management plan",
    "search_text": "exertional chest discomfort cardiac risk ECG troponin acute coronary syndrome"
  }
]
\end{lstlisting}
\end{codebox}

\section{Scoring Rubric and Metric Details}
\label{app:scoring}

This appendix expands the scoring rules and metric definitions used in Section~\ref{sec:statistical_evaluation}. The main paper reports the core quantities; this appendix provides the rubric levels, default parameters, process definitions, longitudinal notation, and sensitivity settings.

\subsection{Outcome rubric}

Diagnostic quality is graded on five levels:
\[
S_i^{\mathrm{diag}}\in\{1.00,0.75,0.50,0.25,0.00\}.
\]
The levels correspond to an exact or clinically equivalent diagnosis, a mostly correct diagnosis with minor deviation, a partially correct diagnosis with moderate omission or bias, a limited but non-dangerous error, and a dangerous or clearly wrong diagnosis. The grading criteria and their clinical interpretation were checked by a professional physician.

Evidence consistency compares the final supporting evidence with manager-side key evidence points. Let $K_i^{\mathrm{evi}}$ be the number of key evidence points, $m_i^{\mathrm{evi}}$ the number of correctly matched points, and $h_i^{\mathrm{evi}}$ the number of contradicted, hallucinated, or unsupported evidence points. We define
\begin{equation*}
S_i^{\mathrm{evi}}
=
\max\left(
0,
\frac{
m_i^{\mathrm{evi}}
-
\lambda_{\mathrm{evi}}h_i^{\mathrm{evi}}
}{
K_i^{\mathrm{evi}}
}
\right).
\end{equation*}

Management quality is scored in the same way. Let $K_i^{\mathrm{plan}}$ be the number of expected management points, $m_i^{\mathrm{plan}}$ the number of matched points, and $h_i^{\mathrm{plan}}$ the number of unsafe or clearly wrong management points. We define
\begin{equation*}
S_i^{\mathrm{plan}}
=
\max\left(
0,
\frac{
m_i^{\mathrm{plan}}
-
\mu_{\mathrm{plan}}h_i^{\mathrm{plan}}
}{
K_i^{\mathrm{plan}}
}
\right).
\end{equation*}

Strict accuracy is computed after diagnosis normalization. Let $\hat{y}_i$ be the raw final diagnosis, $\tilde{y}_i$ its normalized label, and $\mathcal{Y}_i^{\mathrm{acc}}$ the acceptable reference diagnosis set:
\begin{equation*}
A_i^{\mathrm{strict}}
=
\mathbf{1}\{\tilde{y}_i\in\mathcal{Y}_i^{\mathrm{acc}}\}.
\end{equation*}
Pass rate uses the composite score threshold:
\begin{equation*}
P_i=\mathbf{1}\{S_i\geq\tau_{\mathrm{pass}}\}.
\end{equation*}

\subsection{Default parameters}

\begin{table}[!htbp]
\centering
\caption{Default scoring and utility parameters.}
\label{tab:app_default_params}
\small
\begin{tabular}{lc}
\toprule
Parameter & Value \\
\midrule
Outcome weights $(w_{\mathrm{diag}},w_{\mathrm{evi}},w_{\mathrm{plan}})$ & $(0.5,0.3,0.2)$ \\
Evidence penalty $\lambda_{\mathrm{evi}}$ & 0.5 \\
Management penalty $\mu_{\mathrm{plan}}$ & 1.0 \\
Pass threshold $\tau_{\mathrm{pass}}$ & 0.7 \\
Utility weights $(w_1,w_2,w_3,w_4)$ & $(0.6,0.2,0.1,0.1)$ \\
Default maximum turns and tests & $T_{\max}=10$, $E_{\max}=3$ \\
\bottomrule
\end{tabular}
\end{table}

With these parameters, the composite outcome score is
\begin{equation*}
S_i
=
w_{\mathrm{diag}}S_i^{\mathrm{diag}}
+
w_{\mathrm{evi}}S_i^{\mathrm{evi}}
+
w_{\mathrm{plan}}S_i^{\mathrm{plan}},
\end{equation*}
and the utility score is
\begin{equation*}
U_i
=
w_1S_i
-
w_2\frac{T_i}{T_{\max}}
-
w_3\frac{E_i}{E_{\max}}
-
w_4R_i.
\end{equation*}

\subsection{Process metrics}

The event log records each action before finalization. The interaction count is
\begin{equation*}
T_i
=
\#\texttt{ASK}
+
\#\texttt{REQUEST\_TEST}
+
\#\texttt{CALL\_MDT},
\end{equation*}
where $\#\texttt{CALL\_MDT}=0$ when consultation is disabled. The examination count is
\begin{equation*}
E_i=\#\texttt{REQUEST\_TEST}.
\end{equation*}
Let $I_i$ be the number of invalid examination requests, including unavailable tests, unparseable test names, repeated low-value tests, or requests that do not return new information. The invalid-test rate is
\begin{equation*}
R_i
=
\begin{cases}
I_i/E_i, & E_i>0,\\
0, & E_i=0.
\end{cases}
\end{equation*}

\subsection{Longitudinal metrics}

For a staged stream $W_1,\ldots,W_M$, the stage mean of metric $Z$ is
\begin{equation*}
\bar{Z}_m
=
\frac{1}{|W_m|}
\sum_{i\in W_m}
Z_i.
\end{equation*}
The early and late averages used for learning gain are
\begin{equation*}
\bar{Z}_{\mathrm{early}}
=
\frac{1}{|\mathcal{M}_{\mathrm{early}}|}
\sum_{m\in\mathcal{M}_{\mathrm{early}}}
\bar{Z}_m,
\qquad
\bar{Z}_{\mathrm{late}}
=
\frac{1}{|\mathcal{M}_{\mathrm{late}}|}
\sum_{m\in\mathcal{M}_{\mathrm{late}}}
\bar{Z}_m.
\end{equation*}
Thus,
\begin{equation*}
\mathrm{LG}(Z)=\bar{Z}_{\mathrm{late}}-\bar{Z}_{\mathrm{early}}.
\end{equation*}

For held-out transfer, $H_0$ and $H_3$ are evaluated on the same held-out set $\mathcal{H}$. This 100-case held-out set is not used during longitudinal-stream memory accumulation. $H_0$ runs these unseen cases without loading the mature memory bank, whereas $H_3$ runs the same cases after loading the mature memory accumulated from the longitudinal stream. Thus, $\mathrm{ET}(Z)$ isolates external transfer from the fixed-stream replay gains observed in E0--E3:
\begin{equation*}
\mathrm{ET}(Z)
=
\frac{1}{|\mathcal{H}|}
\sum_{i\in\mathcal{H}}
\left(
Z_i^{(H_3)}
-
Z_i^{(H_0)}
\right).
\end{equation*}
The direction of interpretation depends on the metric. Positive values are favorable for higher-is-better metrics such as $S$, $U$, strict accuracy, and pass rate. Negative values are favorable for cost metrics such as $T$ and $E$.

For retention analysis, $A_{k,j}^{(Z)}$ denotes performance on stage $j$ after the system has been updated through stage $k$. For higher-is-better metrics,
\begin{equation*}
\mathrm{BWT}(Z)
=
\frac{1}{K-1}
\sum_{j=1}^{K-1}
\left(
A_{K,j}^{(Z)}
-
A_{j,j}^{(Z)}
\right).
\end{equation*}
Negative BWT indicates backward degradation.

\subsection{Update-stage response}

When a stream contains an explicit update interval, let $\mathcal{M}_{\mathrm{pre}}$, $\mathcal{M}_{\mathrm{upd}}$, and $\mathcal{M}_{\mathrm{post}}$ denote stages before, during, and after the update. For metric $Z$,
\begin{equation*}
\Delta_{\mathrm{upd}}(Z)
=
\bar{Z}_{\mathrm{upd}}
-
\bar{Z}_{\mathrm{pre}},
\qquad
\Delta_{\mathrm{post}}(Z)
=
\bar{Z}_{\mathrm{post}}
-
\bar{Z}_{\mathrm{upd}}.
\end{equation*}
If $\bar{Z}_{\mathrm{upd}}<\bar{Z}_{\mathrm{pre}}$ for a higher-is-better metric, recovery is summarized as
\begin{equation*}
\rho_{\mathrm{recovery}}(Z)
=
\frac{
\bar{Z}_{\mathrm{post}}
-
\bar{Z}_{\mathrm{upd}}
}{
\bar{Z}_{\mathrm{pre}}
-
\bar{Z}_{\mathrm{upd}}
}.
\end{equation*}
This ratio is only interpreted when the update interval produces a drop.

\subsection{Statistical tests}

For two paired conditions $A$ and $B$, continuous or ordinal metrics are compared using case-level differences
\[
d_i^{(Z)}=Z_i^{(B)}-Z_i^{(A)}
\]
on the same case. We report the mean paired difference and use Wilcoxon signed-rank tests. For paired binary outcomes, such as strict correctness and pass/fail status, we use exact McNemar tests. Bootstrap confidence intervals are computed by resampling cases with replacement while preserving the paired structure.

For stage sequences, Mann--Kendall tests summarize monotonic trends, augmented Dickey--Fuller tests summarize stationarity, CUSUM curves identify possible change points, and segmented regression describes slope changes or plateau behavior. These analyses are descriptive diagnostics for longitudinal behavior.

\subsection{Sensitivity}

The main paper reports component metrics alongside composite scores so that conclusions are not determined by a single weighting choice. As a sensitivity check, we recompute utility rankings under alternative cost weights while keeping the same episode logs and outcome scores. Table~\ref{tab:app_utility_sensitivity} reports the resulting rankings.

\begin{table}[!htbp]
\centering
\caption{Utility-weight sensitivity on the 80-case model-comparison subset. Weights are $(S,\mathrm{turns},\mathrm{tests},\mathrm{invalid})$.}
\label{tab:app_utility_sensitivity}
\scriptsize
\setlength{\tabcolsep}{3pt}
\begin{tabular}{lclccc}
\toprule
Setting & Weights & Rank 1 & Rank 2 & Rank 3 & Rank 4 \\
\midrule
Default & $(0.6,0.2,0.1,0.1)$ & GLM-5 & Kimi-K2.5 & Qwen3.5-122B-A10B & Qwen-Turbo \\
Outcome-heavy & $(0.8,0.1,0.1,0.0)$ & GLM-5 & Kimi-K2.5 & Qwen3.5-122B-A10B & Qwen-Turbo \\
Turn-cost-heavy & $(0.4,0.4,0.1,0.1)$ & GLM-5 & Kimi-K2.5 & Qwen-Turbo & Qwen3.5-122B-A10B \\
Test-cost-heavy & $(0.5,0.1,0.3,0.1)$ & GLM-5 & Qwen3.5-122B-A10B & Kimi-K2.5 & Qwen-Turbo \\
Invalid-heavy & $(0.5,0.1,0.1,0.3)$ & GLM-5 & Kimi-K2.5 & Qwen3.5-122B-A10B & Qwen-Turbo \\
\bottomrule
\end{tabular}
\end{table}

\clearpage
\section{Reproducibility Notes, Additional Results, and Ablations}
\label{app:stat_results}

This appendix consolidates the reproduction notes and supplementary experimental results for Section~\ref{sec:experiments}. The results are organized by their role in the paper: model-comparison supplements, MDT consultation supplements, longitudinal memory and held-out transfer, update and retention diagnostics, and memory ablations. Exact split membership, commands, and configuration files are provided in the released artifact rather than duplicated as paper-side command or configuration listings.

\subsection{Reproducibility and Operational Notes}
\label{app:splits_repro}

\paragraph{Reproducibility notes.}
The experiments use API-based inference rather than local model training or fine-tuning. The default random seed is 7. The reported experiments use Qwen-Turbo, Qwen3.5-122B-A10B, GLM-5, and Kimi-K2.5 as doctor, consultant, patient, or manager models depending on the study. Tables in the main paper and appendix report the episode counts used for each study, and configuration files specify the model roles, resource limits, memory mode, and retrieval settings. The reported experiments used API-based inference with an approximate total operational cost of about USD 100 under our provider configuration. Because pricing and routing vary across providers, we report this as an approximate operational cost rather than a standardized benchmark cost; future releases should include standardized per-run cost accounting.

\paragraph{Operational parsing and interaction noise.}
The runner uses JSON-only prompts together with schema and action validation. Malformed or unusable LLM turns are logged as \texttt{llm\_error\_turns}, and invalid catalog requests are logged as \texttt{invalid\_tests} and included in the invalid-test rate. Table~\ref{tab:app_operational_noise} reports these logged noise fields rather than silently dropping them. We do not treat this as a full audit of simulator hallucination or parser-recovery behavior; those remain useful targets for future benchmark hardening.

\begin{table}[!htbp]
\centering
\caption{Logged parsing and interaction-noise indicators.}
\label{tab:app_operational_noise}
\scriptsize
\setlength{\tabcolsep}{2.8pt}
\begin{tabular}{@{}p{0.22\linewidth}ccccc@{}}
\toprule
Study & Records & Error records & Error turns & Invalid tests & Mean invalid \\
\midrule
Exp1 model comparison & 320 & 25.6\% & 291 & 75 & 0.082 \\
Exp2 MDT & 300 & 1.3\% & 5 & 37 & 0.067 \\
Exp3 memory/transfer & 2200 & 4.8\% & 313 & 825 & 0.156 \\
\bottomrule
\end{tabular}
\end{table}

\subsection{Model-Comparison Supplements}
\label{app:model_comparison_supp}

This subsection supports the model-comparison experiment in Section~\ref{sec:experiments}. The paired deltas test whether differences relative to Qwen-Turbo remain visible on the same 80 cases; the confidence-interval table adds uncertainty estimates; the full-vignette comparison provides a static complete-input supplement; and the full summary plus figure decompose outcome and process behavior.

\begin{table}[!htbp]
\centering
\caption{Paired model-comparison deltas against Qwen-Turbo on 80 shared cases. Continuous metrics use Wilcoxon signed-rank tests; strict accuracy uses exact McNemar tests.}
\label{tab:app_model_pairwise}
\scriptsize
\setlength{\tabcolsep}{3pt}
\resizebox{\linewidth}{!}{%
\begin{tabular}{lccccc}
\toprule
Model & $\Delta S$ (95\% CI) & $p_S$ & $\Delta U$ (95\% CI) & $p_U$ & $\Delta$ strict / $p$ \\
\midrule
Qwen3.5-122B-A10B & $+0.074$ [$+0.007,+0.143$] & 0.0783 & $+0.017$ [$-0.026,+0.062$] & 0.581 & $+0.050$ / 0.424 \\
GLM-5 & $+0.318$ [$+0.258,+0.377$] & $1.78{\times}10^{-12}$ & $+0.193$ [$+0.154,+0.232$] & $9.24{\times}10^{-12}$ & $+0.275$ / $2.74{\times}10^{-5}$ \\
Kimi-K2.5 & $+0.275$ [$+0.214,+0.339$] & $3.03{\times}10^{-10}$ & $+0.114$ [$+0.072,+0.157$] & $1.27{\times}10^{-5}$ & $+0.163$ / 0.00443 \\
\bottomrule
\end{tabular}
}
\end{table}

\begin{table}[!htbp]
\centering
\caption{Answer-only and episode-trace model-comparison summary with 95\% bootstrap CIs. Answer-only metrics are projections from the final answer produced during the episode; trace metrics additionally provide utility and process costs.}
\label{tab:app_static_dynamic_ci}
\scriptsize
\setlength{\tabcolsep}{3pt}
\begin{tabular}{lcccccc}
\toprule
Model & Ans. strict & Ans. $S$ & Trace $S$ CI & Trace $U$ & Trace $U$ CI & Invalid \\
\midrule
Qwen-Turbo & 0.100 & 0.304 & [0.261, 0.348] & 0.001 & [-0.029, 0.033] & 0.077 \\
Qwen3.5-122B-A10B & 0.150 & 0.378 & [0.320, 0.438] & 0.018 & [-0.020, 0.060] & 0.010 \\
GLM-5 & 0.375 & 0.622 & [0.565, 0.675] & 0.195 & [0.158, 0.230] & 0.050 \\
Kimi-K2.5 & 0.263 & 0.579 & [0.522, 0.638] & 0.115 & [0.073, 0.158] & 0.192 \\
\bottomrule
\end{tabular}
\end{table}

\begin{table}[!htbp]
\centering
\caption{Full-vignette static QA results and paired dynamic episode comparison on the 80-case subset for two models. Static evaluation gives the complete case vignette in a single prompt and excludes manager-only fields, gold diagnoses, aliases, and rubrics.}
\label{tab:app_full_vignette_static}
\scriptsize
\setlength{\tabcolsep}{3.2pt}
\begin{tabular}{lccccccccc}
\toprule
Model & $N$ & Static strict & Static accept. & Static $S_d$ & Static $S_e$ & Static $S_p$ & Static $S$ & Dyn. strict & Dyn. $S$ \\
\midrule
Qwen-Turbo & 80 & 0.288 & 0.388 & 0.472 & 0.682 & 0.722 & 0.585 & 0.100 & 0.304 \\
Kimi-K2.5 & 80 & 0.125 & 0.625 & 0.581 & 0.836 & 0.922 & 0.726 & 0.263 & 0.579 \\
\bottomrule
\end{tabular}
\end{table}

The static condition is a paired supplement rather than a replacement for episode evaluation. It shows that complete-input final-answer performance and interactive episode performance can differ in both magnitude and direction: Qwen-Turbo improves under full-vignette input, whereas Kimi-K2.5 has a higher static composite score but lower static strict diagnostic accuracy than in the dynamic episode condition. Static QA therefore helps contextualize final-answer ability, while episode traces remain necessary for measuring information acquisition, examination cost, invalid actions, and utility.

\begin{table}[!htbp]
\centering
\caption{Full model-comparison summary on 80 shared episodes.}
\label{tab:app_exp1_full}
\small
\begin{tabular}{lcccccccc}
\toprule
Model & Strict & Accept. & $S_d$ & $S_e$ & $S_p$ & $S$ & Turns & Tests \\
\midrule
Qwen-Turbo & 0.100 & 0.175 & 0.281 & 0.274 & 0.406 & 0.304 & 5.713 & 1.388 \\
Qwen3.5-122B-A10B & 0.150 & 0.275 & 0.322 & 0.433 & 0.434 & 0.378 & 7.975 & 0.900 \\
GLM-5 & 0.375 & 0.525 & 0.572 & 0.614 & 0.759 & 0.622 & 4.463 & 2.225 \\
Kimi-K2.5 & 0.263 & 0.488 & 0.506 & 0.569 & 0.778 & 0.580 & 5.725 & 2.575 \\
\bottomrule
\end{tabular}
\end{table}

\begin{figure}[!htbp]
\centering
\includegraphics[width=\linewidth]{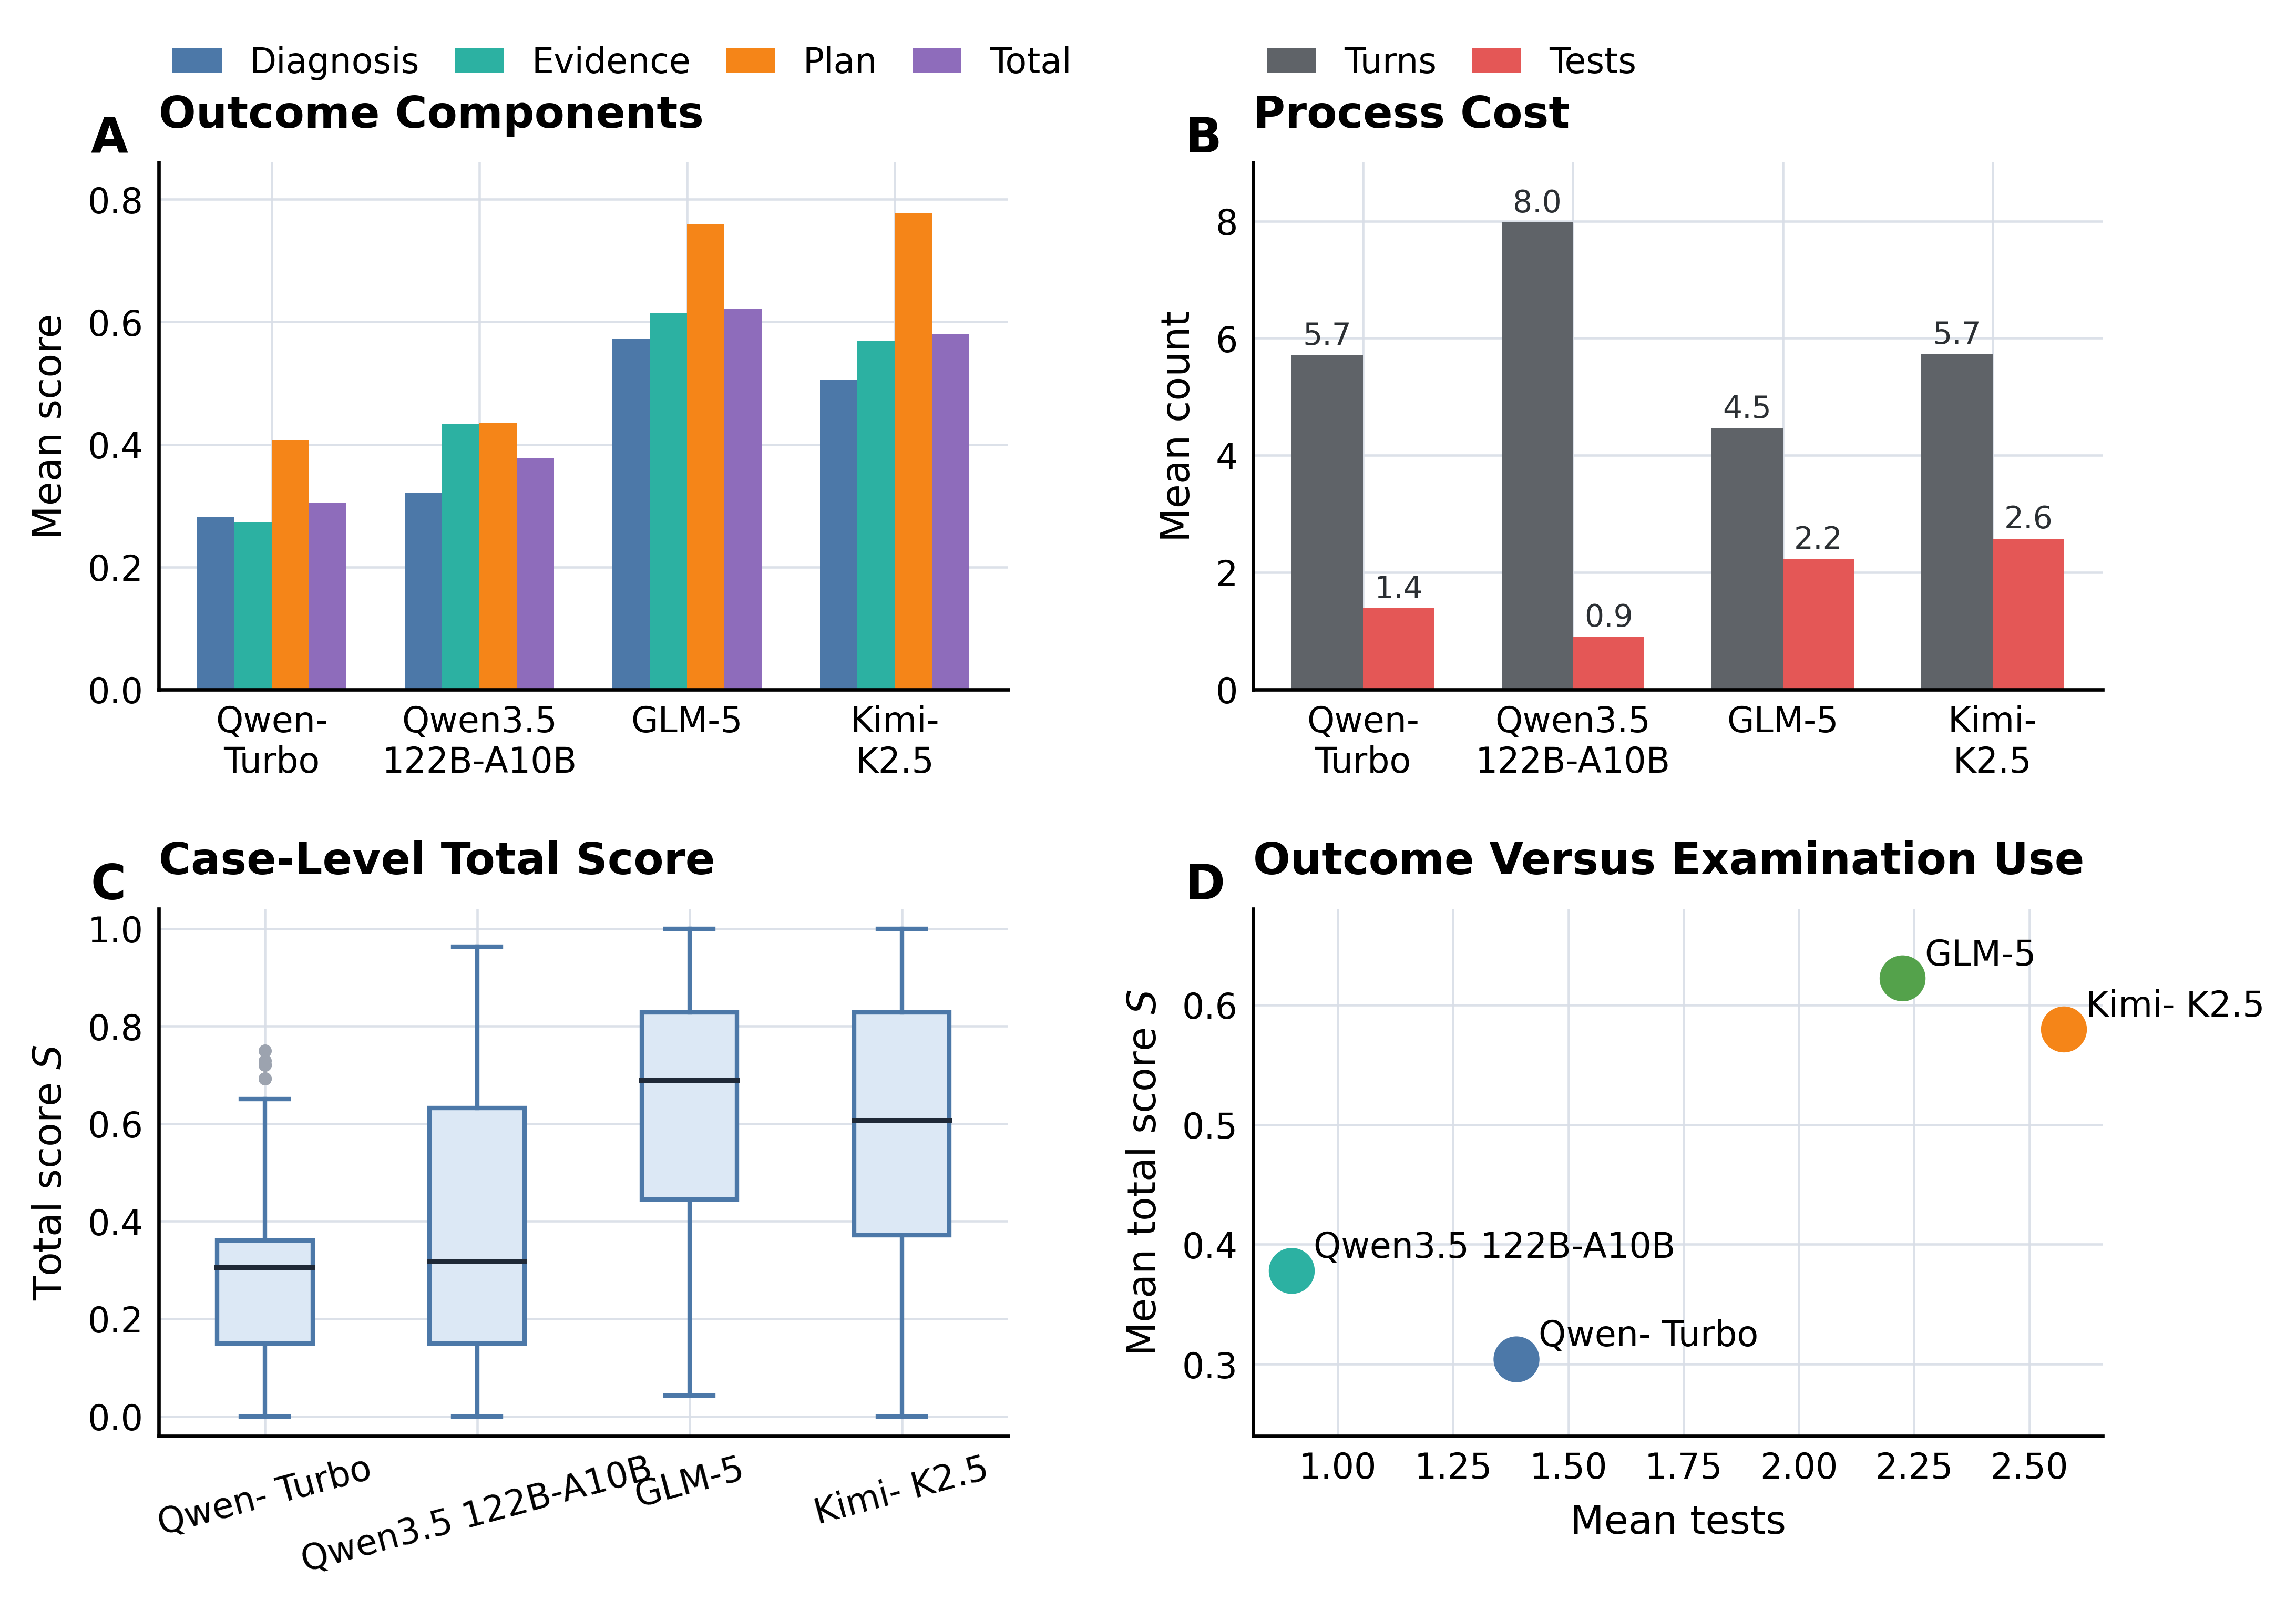}
\caption{Model-comparison evidence on 80 shared episodes. (A) Outcome components separate diagnosis, evidence, plan, and total score. (B) Process cost compares interaction turns and requested tests. (C) Case-level score distributions expose variance across episodes. (D) Outcome-versus-testing view shows that higher total score and higher examination use are not identical.}
\label{fig:app_model_comparison}
\end{figure}

Together, these supplementary results support the main conclusion of Section~\ref{sec:experiments}: the episode trace separates final clinical quality from process cost, examination use, invalid actions, and utility.

\subsection{MDT Consultation Supplements}
\label{app:mdt_full_results}

This subsection supports the MDT experiment. The table gives the full outcome summary, while the figure decomposes whether the intervention changes outcome metrics, consultation behavior, examination use, and diagnosis-change patterns.

\begin{table}[!htbp]
\centering
\caption{Full MDT summary on 100 shared episodes.}
\label{tab:app_exp2_full}
\small
\begin{tabular}{lccccccc}
\toprule
Setting & Strict & Accept. & $S_d$ & $S_e$ & $S_p$ & $S$ & Tests \\
\midrule
No MDT & 0.100 & 0.180 & 0.303 & 0.283 & 0.391 & 0.303 & 1.37 \\
Same-model MDT & 0.080 & 0.130 & 0.270 & 0.276 & 0.378 & 0.284 & 0.66 \\
Stronger-consultant MDT & 0.070 & 0.140 & 0.278 & 0.299 & 0.395 & 0.293 & 0.63 \\
\bottomrule
\end{tabular}
\end{table}

\begin{figure}[!htbp]
\centering
\includegraphics[width=\linewidth]{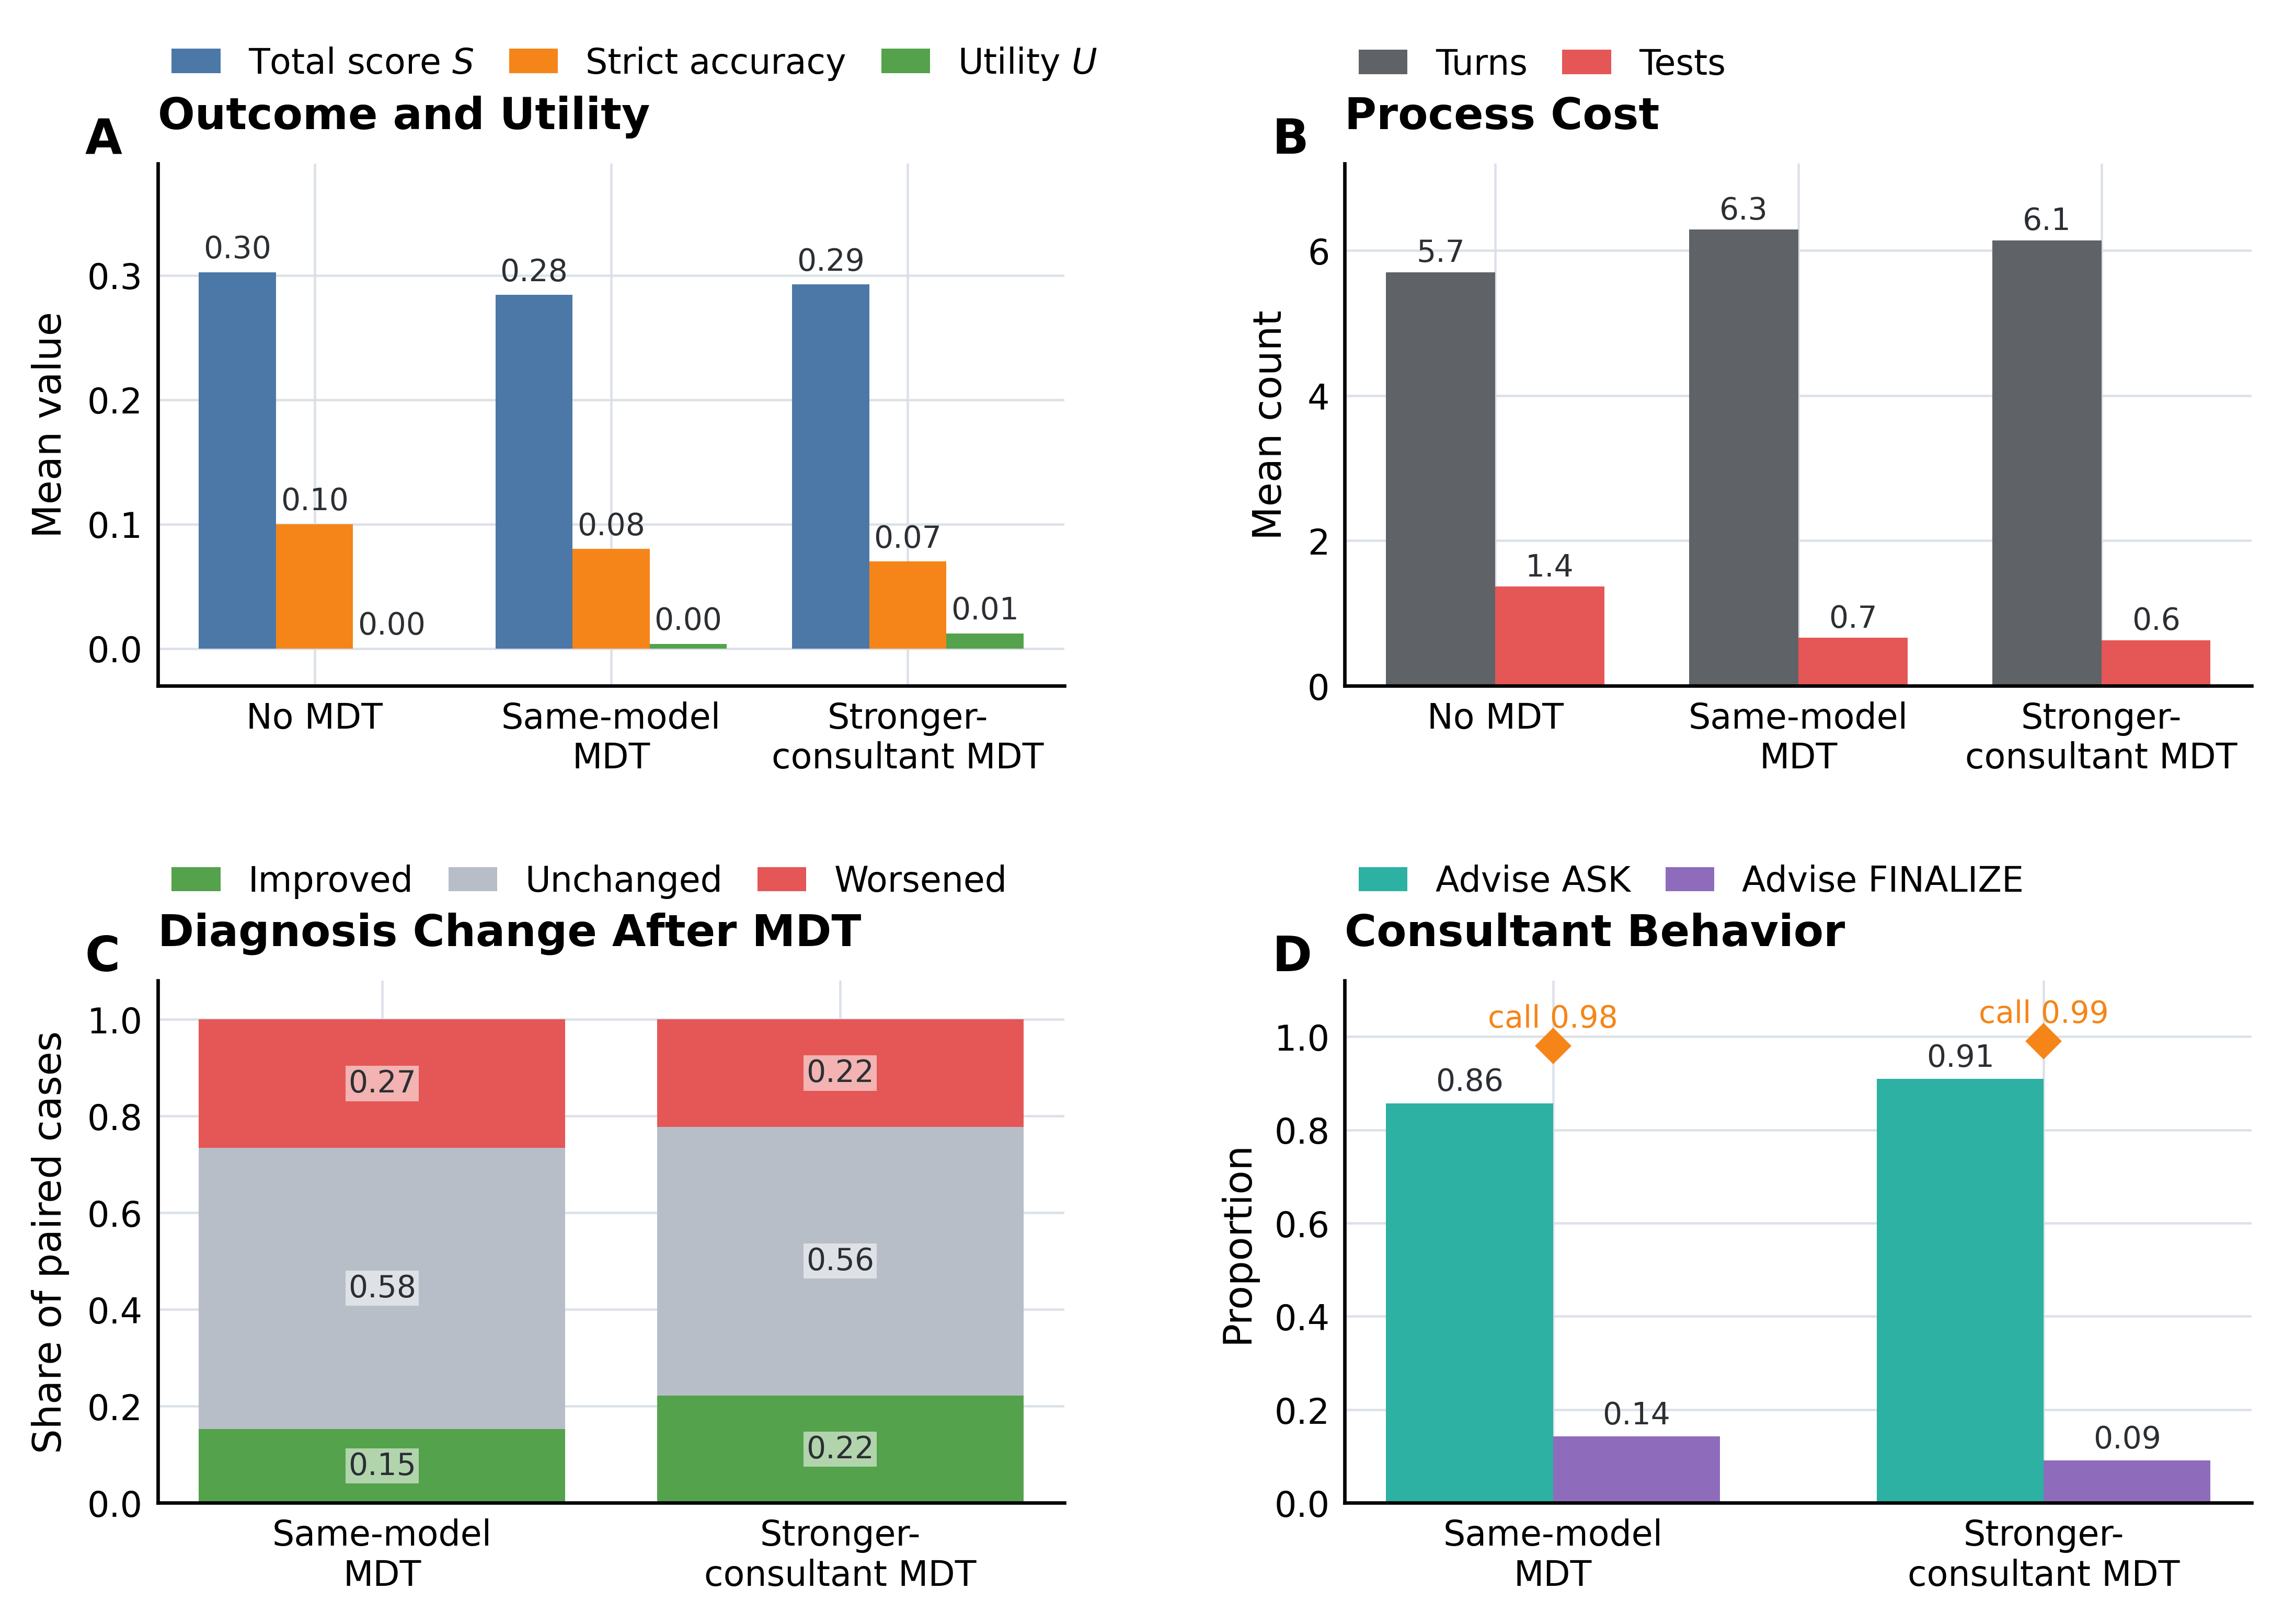}
\caption{MDT decomposition on 100 shared episodes. (A) Outcome and utility compare no MDT, same-model consultation, and stronger-consultant consultation. (B) Process cost shows the trade-off between more interaction turns and fewer examinations. (C) Diagnosis-change ratios identify whether MDT improves, preserves, or worsens paired cases. (D) Consultant behavior reports advice patterns together with call rates.}
\label{fig:app_mdt_analysis}
\end{figure}

The supplementary MDT results support the interpretation in the main paper: in this Qwen-Turbo primary-doctor setting, consultation mainly shifts process effort away from examinations and toward consultation turns, while strict diagnostic accuracy and total score change only slightly.

\subsection{Longitudinal Memory and Held-Out Transfer}
\label{app:memory_transfer_supp}

This subsection supports the longitudinal memory experiment. The first table summarizes the no-memory, cold-start-memory, mature-memory, and held-out transfer conditions. The learning curves then show how the memory pattern varies across stages, and the paired H0/H3 table tests whether mature memory transfers to unseen cases.

\begin{table}[!htbp]
\centering
\caption{Main longitudinal memory summary.}
\label{tab:app_memory_full}
\small
\begin{tabular}{lccccccc}
\toprule
Group & Cases & $S$ & $U$ & Strict & Pass & Turns & Tests \\
\midrule
E0 & 500 & 0.246 & -0.054 & 0.092 & 0.056 & 6.134 & 1.450 \\
E1 & 500 & 0.261 & -0.043 & 0.136 & 0.096 & 6.324 & 1.274 \\
E2 & 500 & 0.377 & 0.037 & 0.276 & 0.244 & 5.696 & 1.370 \\
E3 & 500 & 0.430 & 0.077 & 0.342 & 0.284 & 5.380 & 1.360 \\
H0 & 100 & 0.338 & 0.001 & 0.290 & 0.180 & 6.810 & 1.300 \\
H3 & 100 & 0.413 & 0.068 & 0.330 & 0.260 & 5.820 & 1.410 \\
\bottomrule
\end{tabular}
\end{table}

Stage-level learning curves are generated by the released analysis scripts for total score, utility, exact diagnosis rate, pass rate, turns, and tests. The qualitative pattern is consistent across the main outcome plots: E2 and E3 are above E0 and E1 for most stages, but within-pass stage trends are not monotonically increasing because later windows can be more difficult.

\begin{figure}[!htbp]
\centering
\includegraphics[width=\linewidth]{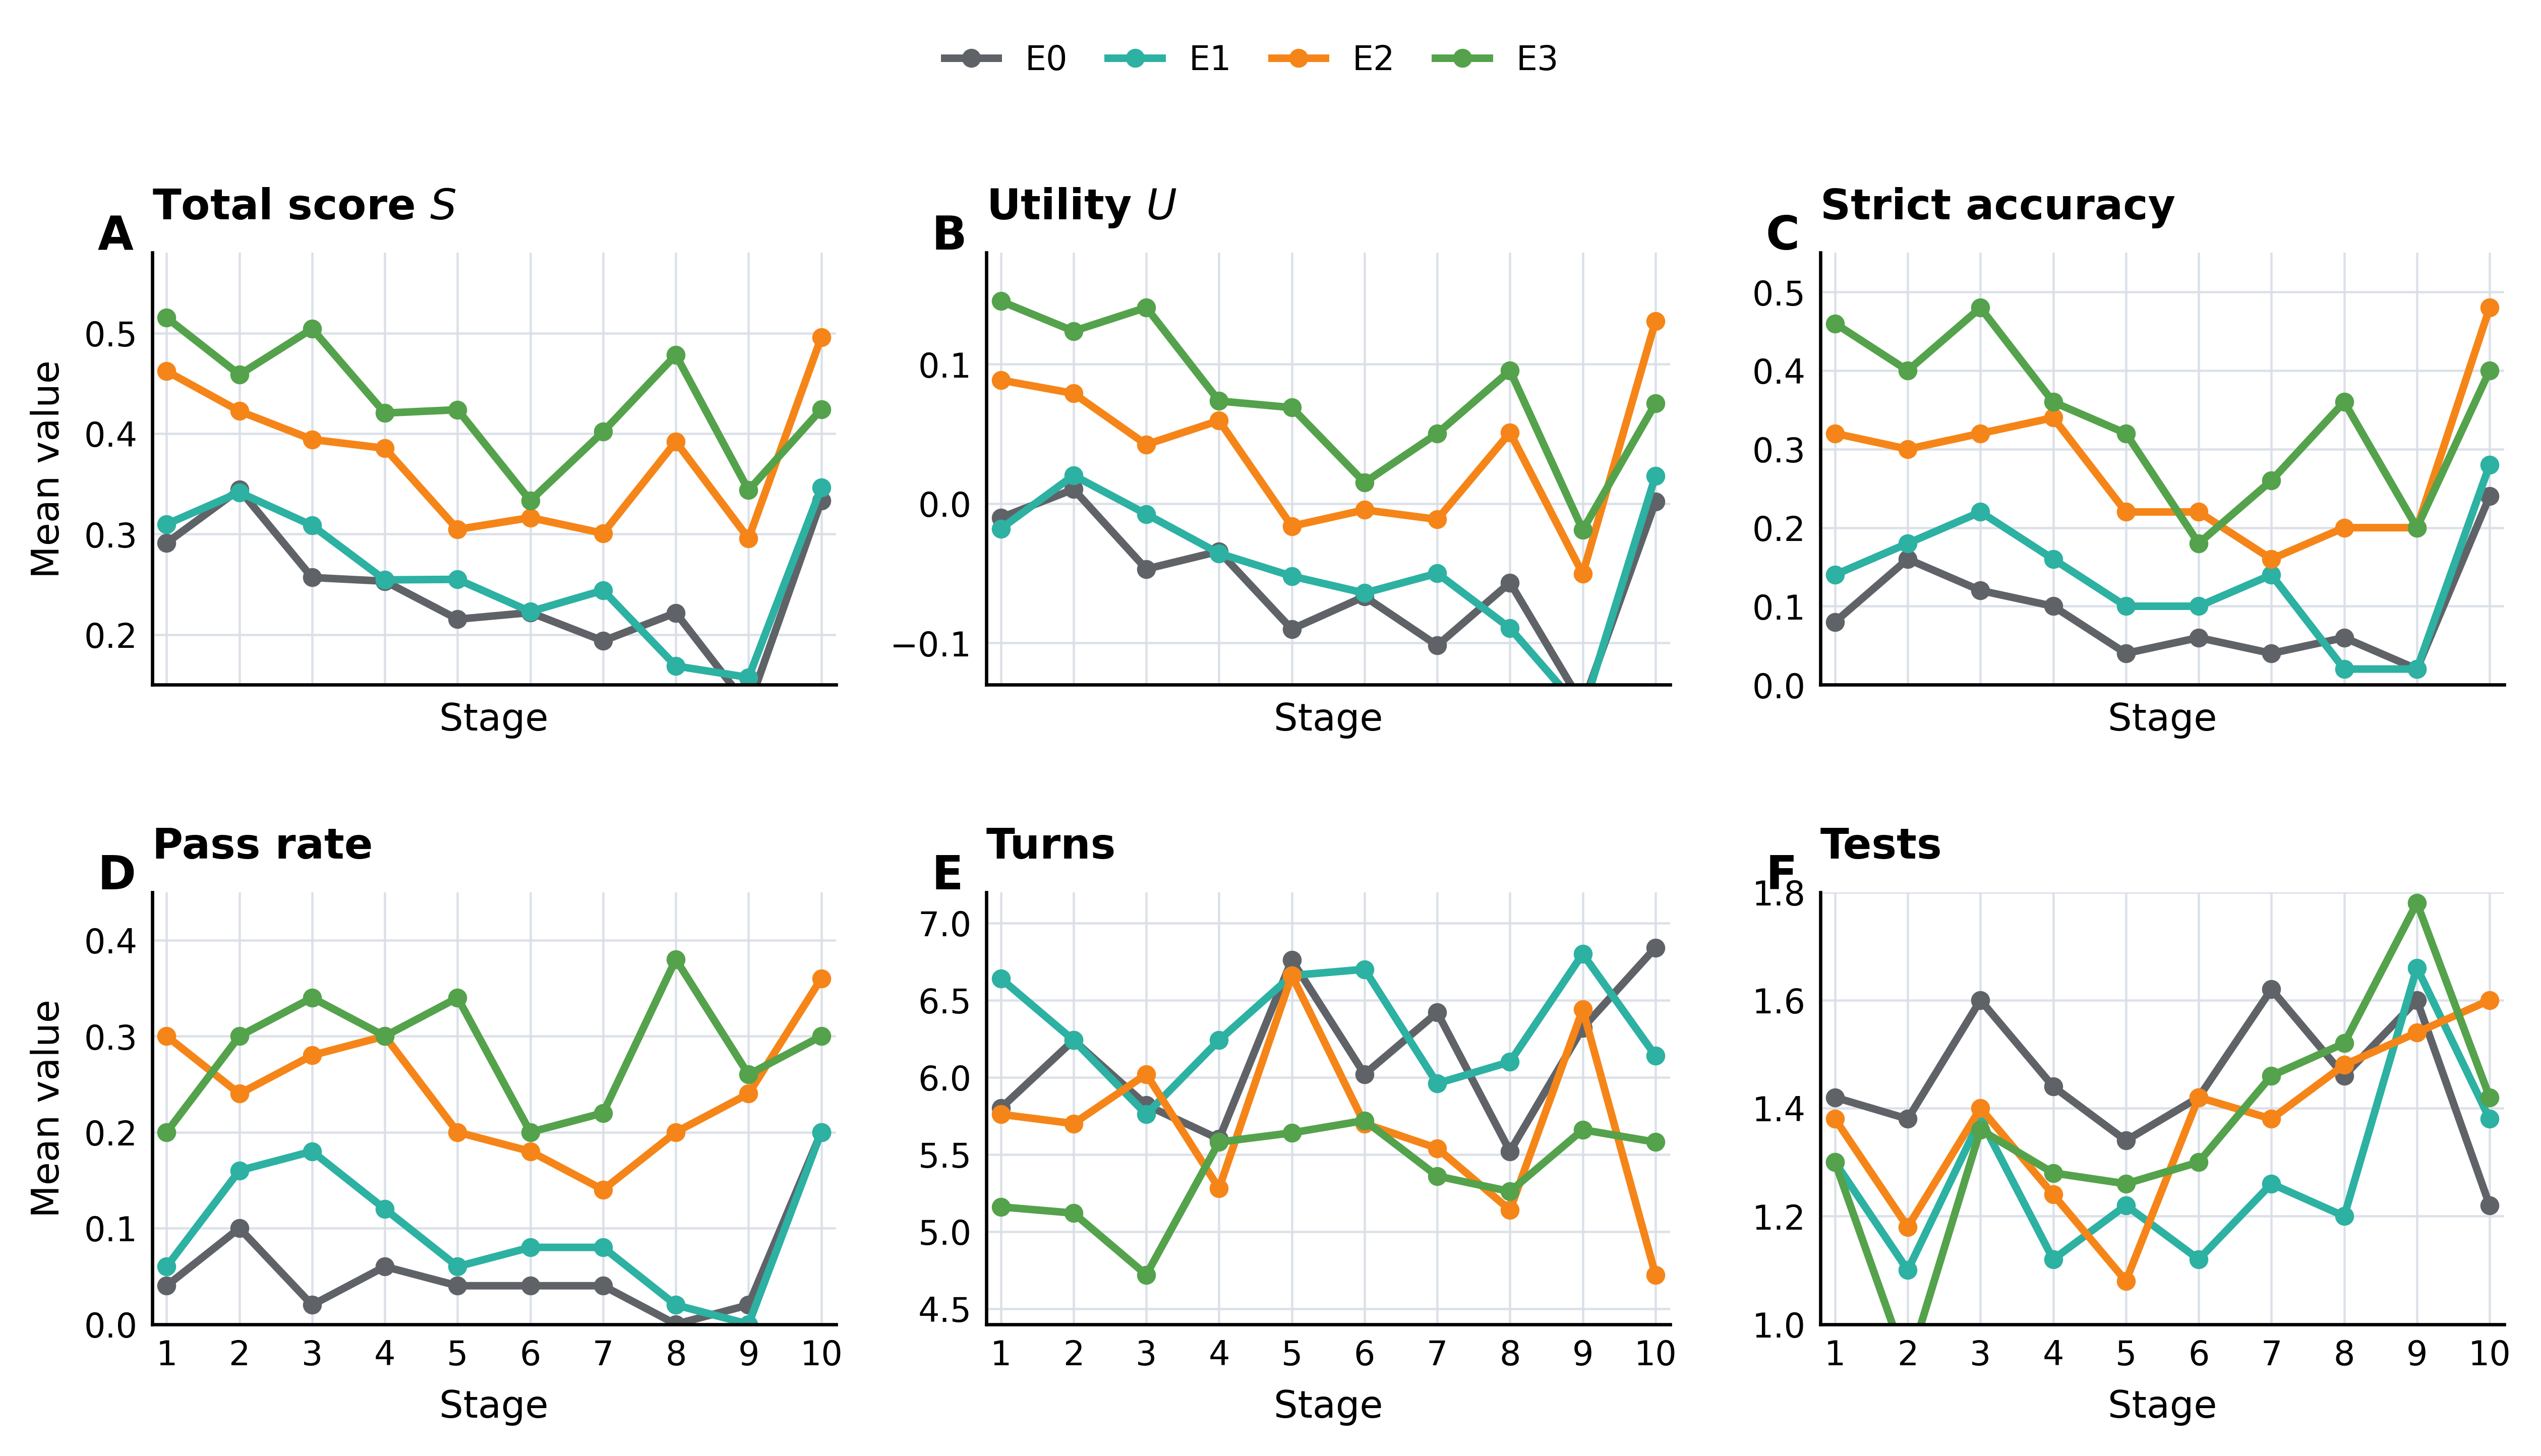}
\caption{Stage-level memory curves. (A) Total score improves mainly after memory matures. (B) Utility follows the same mature-memory pattern while penalizing cost. (C) Strict accuracy rises after E2/E3. (D) Pass rate shows the thresholded outcome gain. (E) Turns decline under mature memory. (F) Tests remain a separate resource signal rather than a direct proxy for score.}
\label{fig:app_learning_curves}
\end{figure}

H0 and H3 are evaluated on the same 100 external holdout cases, which are excluded from the longitudinal stream used to build memory. H0 is the no-mature-memory condition on this held-out set, while H3 loads the mature memory produced after the third longitudinal pass before evaluating the same cases. We therefore report paired Wilcoxon signed-rank tests for continuous or ordinal metrics and exact McNemar tests for paired binary outcomes. The table below is computed from matched H0/H3 case-level records in the experiment outputs and tests external transfer rather than repeated evaluation on the original stream.

\begin{table}[!htbp]
\centering
\caption{Paired comparison on the external holdout set (H0 vs. H3).}
\label{tab:app_h0h3_paired}
\small
\begin{tabular}{lcccl}
\toprule
Metric & H0 & H3 & $\Delta$ & Test \\
\midrule
Total score $S$ & 0.338 & 0.413 & +0.075 & Wilcoxon, $p=0.0408$ \\
Utility $U$ & 0.001 & 0.068 & +0.067 & Wilcoxon, $p=0.00314$ \\
Turns & 6.810 & 5.820 & $-0.990$ & Wilcoxon, $p=0.000231$ \\
Tests & 1.300 & 1.410 & +0.110 & Wilcoxon, $p=0.151$ \\
Strict accuracy & 0.290 & 0.330 & +0.040 & McNemar, $p=0.572$ \\
Pass rate & 0.180 & 0.260 & +0.080 & McNemar, $p=0.152$ \\
Non-dangerous diagnosis & 0.550 & 0.680 & +0.130 & McNemar, $p=0.0351$ \\
\bottomrule
\end{tabular}
\end{table}

\begin{figure}[!htbp]
\centering
\includegraphics[width=\linewidth]{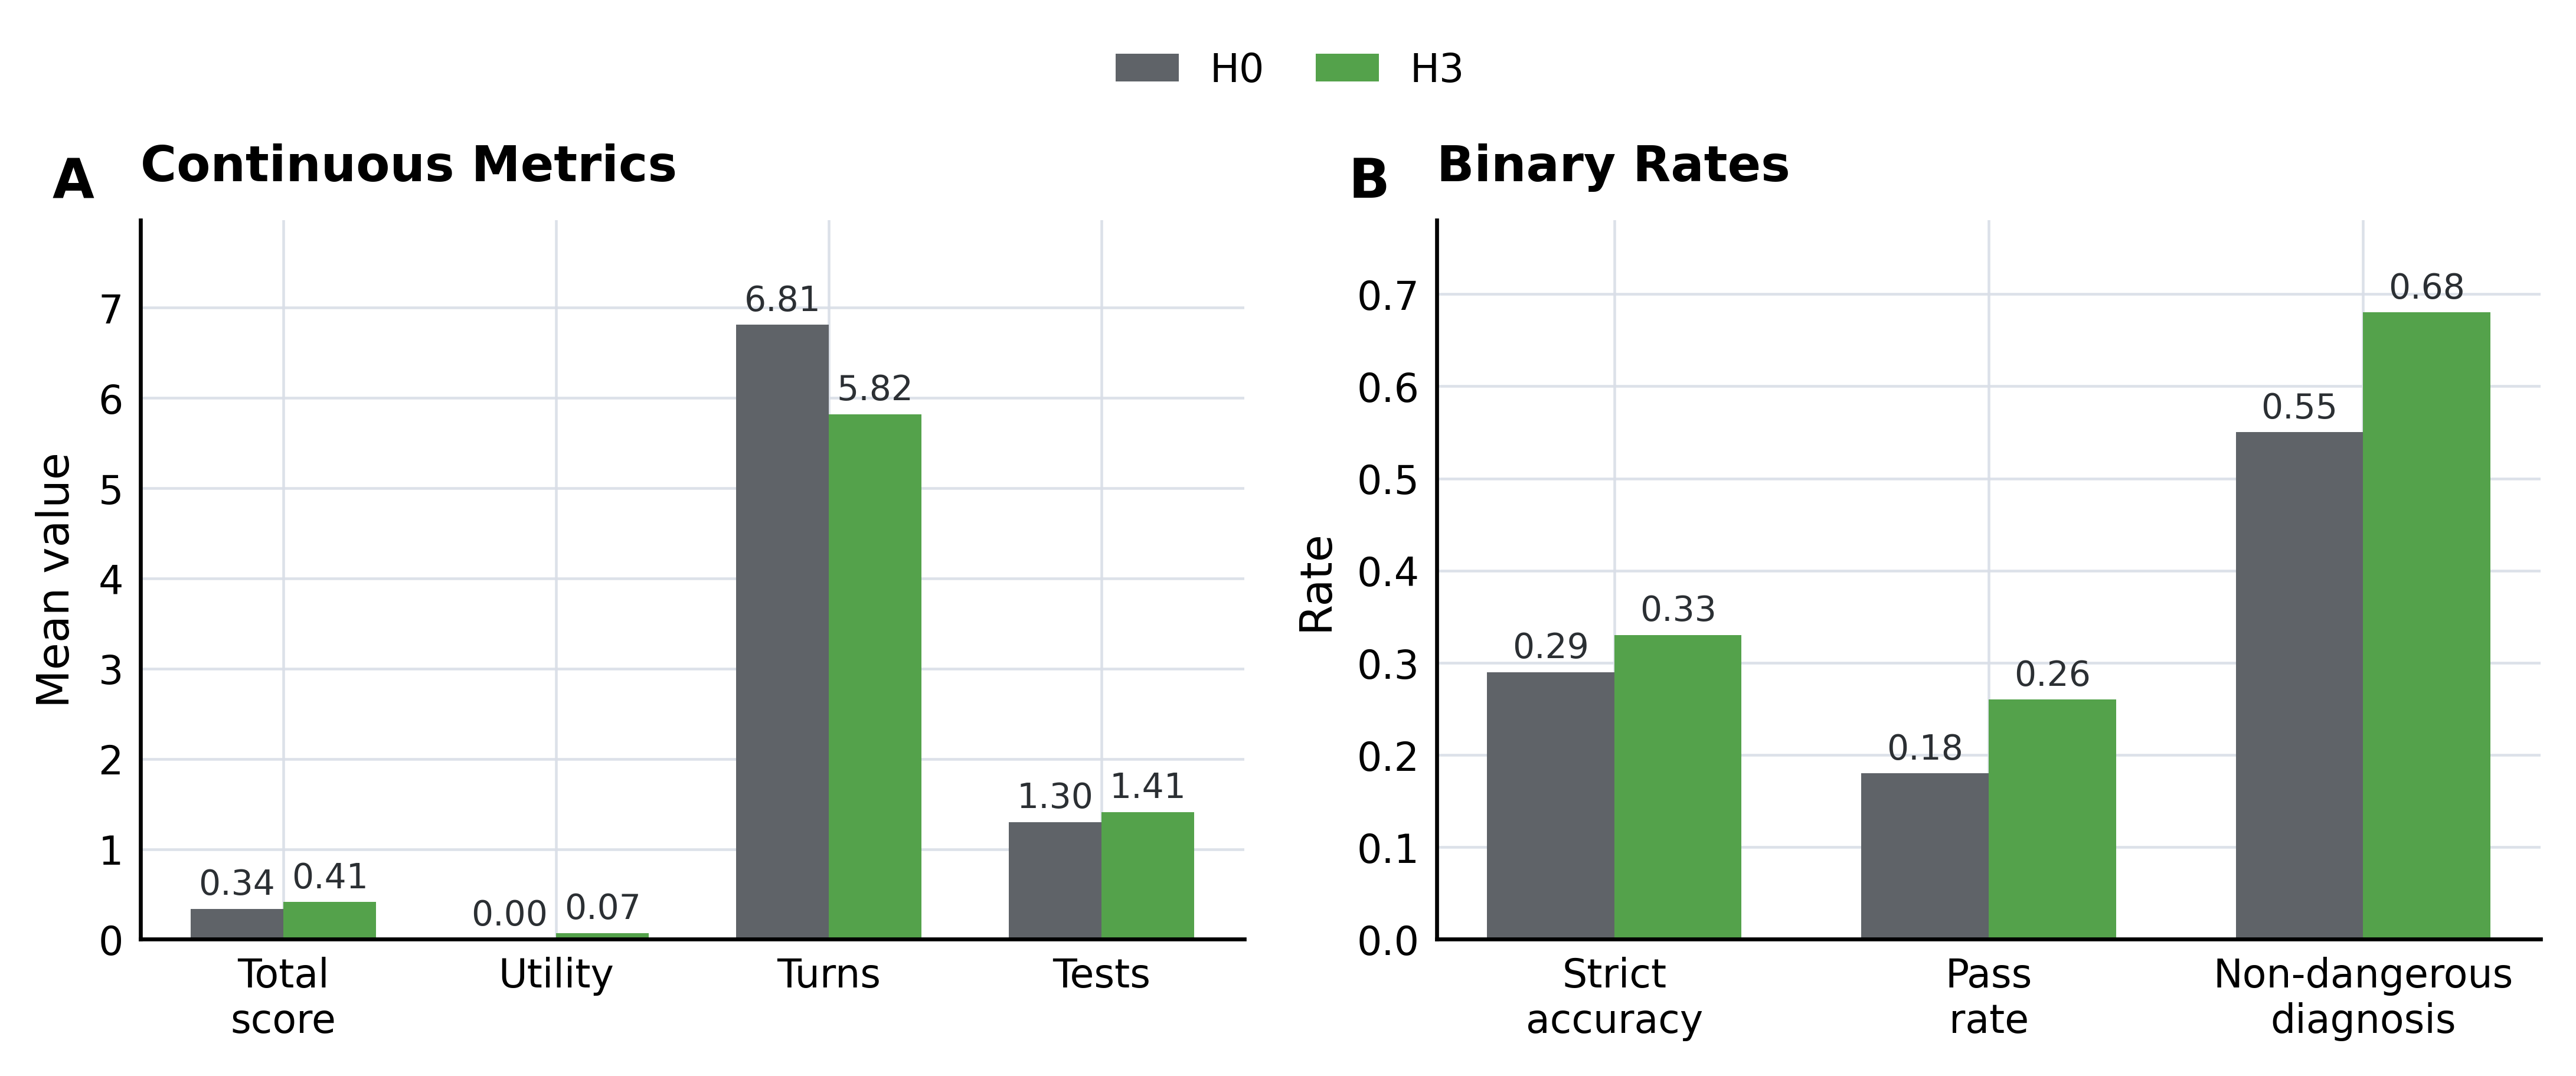}
\caption{External transfer comparison between H0 and H3 on 100 held-out episodes.}
\label{fig:app_external_transfer}
\end{figure}

The longitudinal and held-out results support a memory-maturation interpretation. E1 shows limited cold-start gains, while E2 and E3 show larger gains in outcome and utility. On unseen cases, H3 improves total score and utility and reduces turns, although strict accuracy and pass rate remain weaker binary signals in the 100-case holdout.

\subsection{Update and Retention Diagnostics}
\label{app:update_retention}

This subsection collects diagnostics for the update and retention analysis. The early--late table checks whether within-pass stage means show monotonic improvement, while the update/BWT table and figure separate update-stage response from backward retention.

\begin{table}[!htbp]
\centering
\caption{Early--late stage diagnostics for the main memory stream.}
\label{tab:app_early_late}
\small
\begin{tabular}{lcccc}
\toprule
Group & $S$ early & $S$ late & $U$ early & $U$ late \\
\midrule
E0 & 0.318 & 0.231 & 0.000 & -0.071 \\
E1 & 0.326 & 0.252 & 0.001 & -0.065 \\
E2 & 0.442 & 0.396 & 0.084 & 0.040 \\
E3 & 0.487 & 0.384 & 0.134 & 0.026 \\
\bottomrule
\end{tabular}
\end{table}

\begin{table}[!htbp]
\centering
\caption{Update response and backward-transfer diagnostics.}
\label{tab:app_update_bwt}
\small
\begin{tabular}{lcccc}
\toprule
Group/metric & Pre & Update & Post & Change note \\
\midrule
G0 total score & 0.238 & 0.345 & 0.242 & update response $+0.108$ \\
G0 utility & -0.057 & 0.010 & -0.051 & update response $+0.067$ \\
G1 total score & 0.230 & 0.348 & 0.277 & update response $+0.118$ \\
G1 utility & -0.069 & 0.033 & -0.027 & update response $+0.102$ \\
BWT total score & -- & -- & -- & -0.0087 \\
BWT utility & -- & -- & -- & -0.0103 \\
\bottomrule
\end{tabular}
\end{table}

\paragraph{Descriptive time-series diagnostics.}
Mann--Kendall, ADF, CUSUM, and segmented-regression outputs are treated as descriptive checks rather than definitive significance evidence because update analyses use only ten stage points. In the update experiment, the update windows raise both G0 and G1 means, so the event is interpreted as a distributional response test rather than a purely adverse shock.

\begin{figure}[!htbp]
\centering
\includegraphics[width=\linewidth]{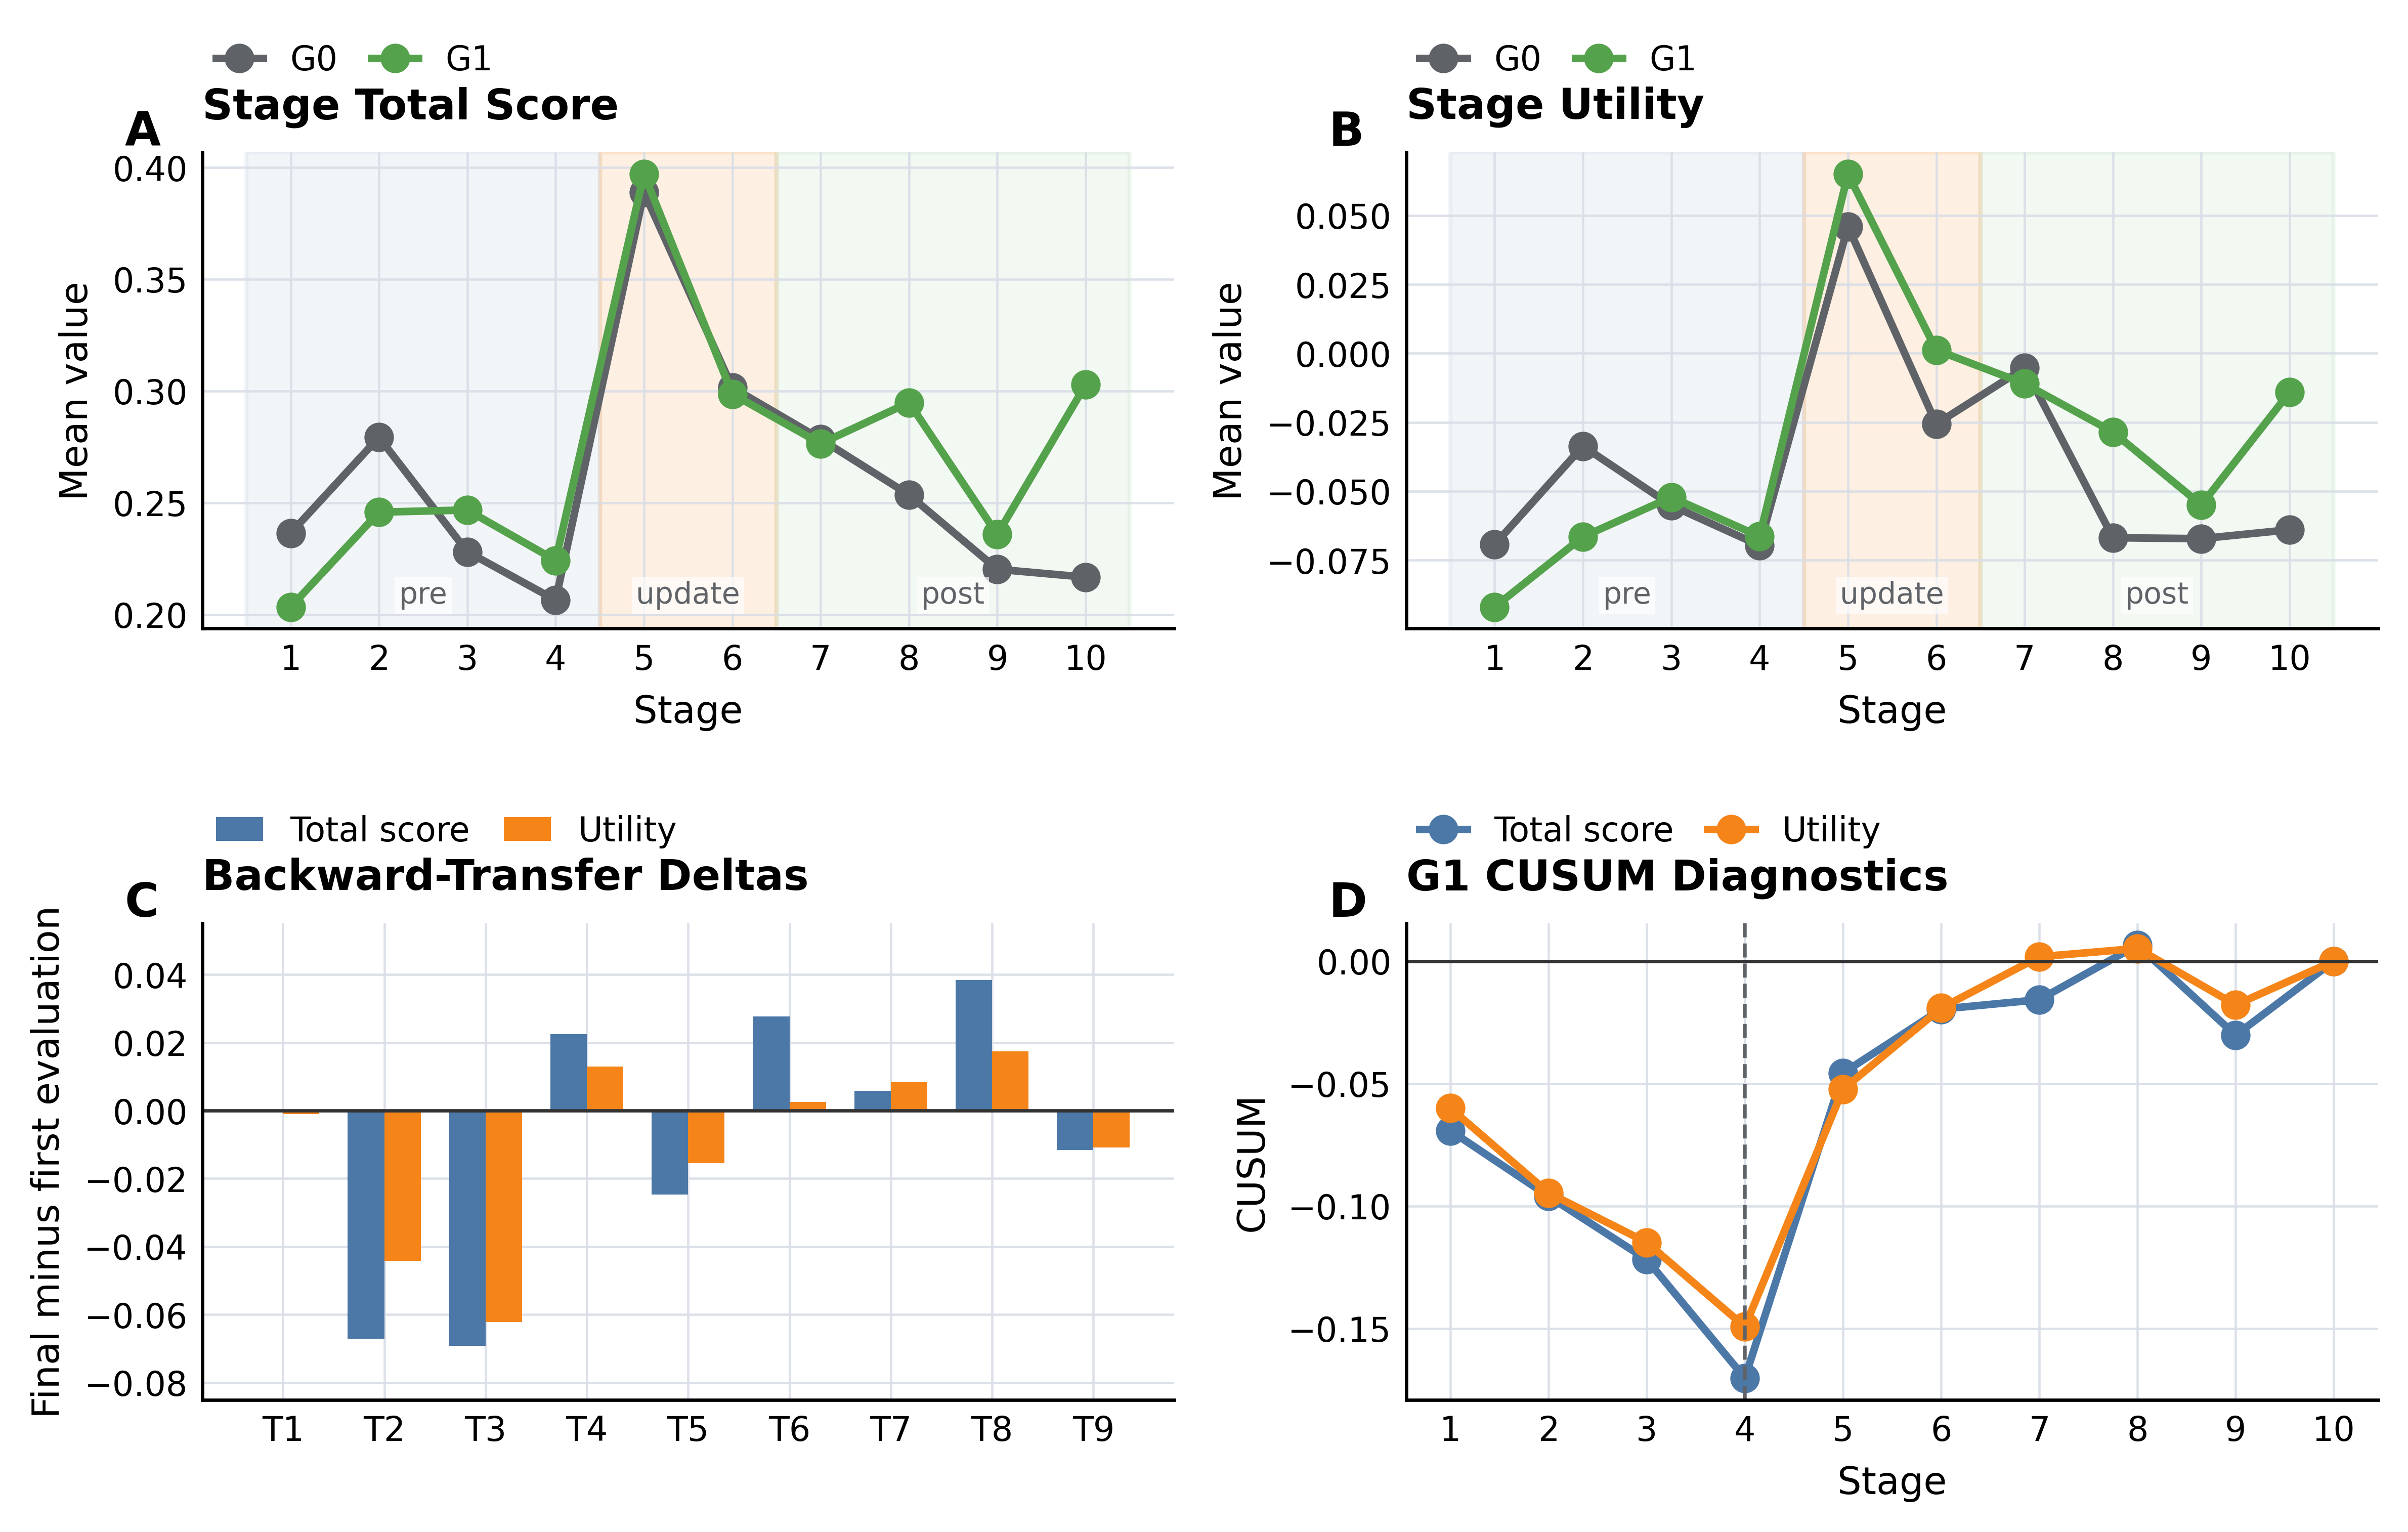}
\caption{Update and retention diagnostics. (A) Stage total score separates pre-update, update, and post-update windows. (B) Stage utility repeats the analysis with resource penalties. (C) Backward-transfer deltas compare final evaluation against first evaluation on earlier stages. (D) G1 CUSUM curves provide a descriptive check for stage-level shifts.}
\label{fig:app_update_diagnostics}
\end{figure}

The update results should therefore be read together with BWT. The update interval produces a positive current-stage response, while the BWT values indicate mild backward degradation rather than catastrophic forgetting.

\subsection{Memory-Content and Retrieval-Scale Ablations}
\label{app:curves_ablations}

This subsection reports mechanism-oriented ablations on a 100-case subset. The memory-content ablation compares success-plus-failure memory with failure-only memory, and the retrieval-scale ablation varies $K_{\mathrm{ret}}$ under the same success-and-failure memory setting.

\begin{figure}[!htbp]
\centering
\includegraphics[width=\linewidth]{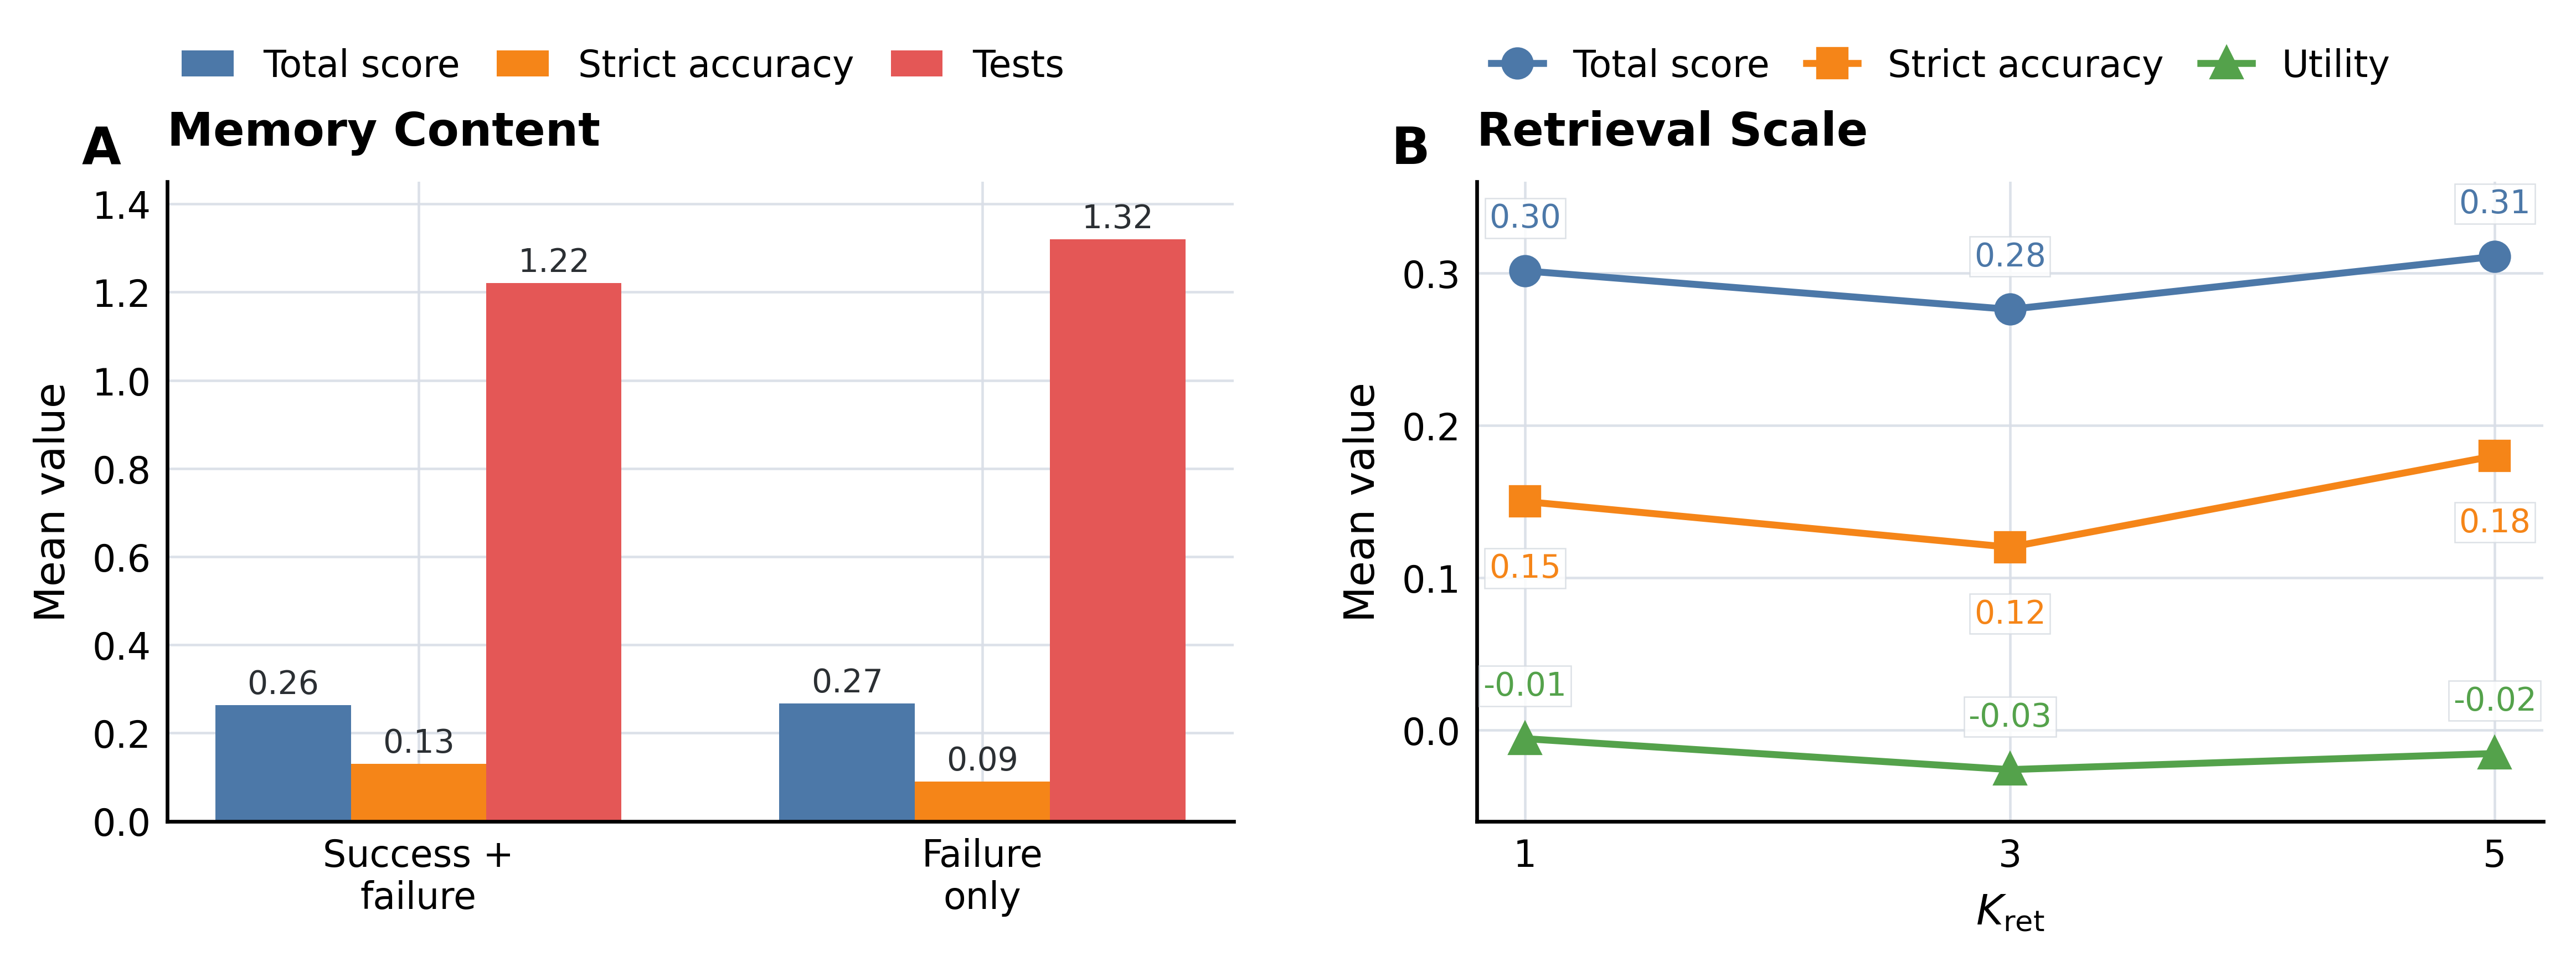}
\caption{Memory ablations on the 100-case mechanism subset. (A) Memory-content comparison tests whether success and failure cards differ from failure-only cards. (B) Retrieval-scale comparison varies $K_{\mathrm{ret}}$ and tracks score, strict accuracy, and utility.}
\label{fig:app_ablation_results}
\end{figure}

\begin{table}[!htbp]
\centering
\caption{Memory-content ablation on the 100-case mechanism subset with $K_{\mathrm{ret}}=3$.}
\label{tab:app_ablation_memory_type}
\small
\begin{tabular}{lcccccc}
\toprule
Memory setting & $S$ & $U$ & Pass & Turns & Tests & Strict \\
\midrule
Success + failure & 0.2627 & -0.0355 & 0.09 & 6.21 & 1.22 & 0.13 \\
Failure only & 0.2668 & -0.0312 & 0.09 & 5.99 & 1.32 & 0.09 \\
\bottomrule
\end{tabular}
\end{table}

\begin{table}[!htbp]
\centering
\caption{Retrieval-scale ablation on the 100-case mechanism subset with success and failure memories enabled.}
\label{tab:app_ablation_topk}
\small
\begin{tabular}{ccccccc}
\toprule
$K_{\mathrm{ret}}$ & $S$ & $U$ & Pass & Turns & Tests & Strict \\
\midrule
1 & 0.3015 & -0.0058 & 0.13 & 5.68 & 1.38 & 0.15 \\
3 & 0.2763 & -0.0261 & 0.08 & 6.28 & 1.21 & 0.12 \\
5 & 0.3110 & -0.0155 & 0.17 & 6.39 & 1.34 & 0.18 \\
\bottomrule
\end{tabular}
\end{table}

These ablations do not identify one setting that dominates every metric. Success memory improves strict diagnosis relative to failure-only memory but does not improve the composite score in this small subset. Retrieval size has a larger effect: $K_{\mathrm{ret}}=5$ gives the best outcome metrics, while $K_{\mathrm{ret}}=1$ gives the best utility and shortest consultations.

\section{Physician Audit and Scorer Validity}
\label{app:llm_sim_audit}

This appendix supplements the automatic-scoring limitation discussed in Section~\ref{sec:discussion_limitations}.

To stress-test manager-side scoring, we performed a single-physician blinded clinical audit on 100 sampled episode final outputs. The sample was stratified across model-comparison and memory/held-out settings, memory and no-memory conditions, correct and incorrect diagnoses, and dangerous and non-dangerous cases. The physician auditor was blinded to the automatic manager scores and reviewed the final diagnosis, evidence, and plan fields against the reference diagnosis and rubric information. The audit protocol was: independent physician grading, post-hoc comparison with manager outputs, disagreement categorization by diagnosis boundary or rubric-coverage issue, and trace-level localization using the final structured output, returned examinations, and matched or missing rubric points.

\begin{table}[!htbp]
\centering
\caption{Single-physician clinical audit summary on 100 sampled final outputs.}
\label{tab:app_llm_sim_audit}
\small
\begin{tabular}{lccccc}
\toprule
Audit source & $N$ & Diagnosis agreement & Diag. kappa & Evidence corr. & Plan corr. \\
\midrule
Blinded physician auditor & 100 & 0.920 & 0.892 & 0.914 & 0.931 \\
\bottomrule
\end{tabular}
\end{table}

Typical disagreements occurred near boundary diagnosis grades and rubric-coverage judgments, especially when a final answer named a related disease family but omitted decisive evidence or management details. This audit measures manager-vs.-physician agreement for automatic scoring. It does not estimate agreement among multiple physicians, and larger physician-adjudicated subsets remain important future work.
